# Supplementary material for: Fusing machine learning strategy with density functional theory to hasten the discovery of MXenes for hydrogen generation
Source: arXiv:2212.05213 source file (2022-12-10)
Supplement: Supplementary file 1 [file preprint-SI.pdf]

## Supplementary Information

### **Fusing machine learning strategy with density functional theory to hasten the discovery of MXenes for hydrogen generation**

B. Moses Abraham<sup>1†</sup>, Priyanka Sinha<sup>1†</sup>, Prosun Halder<sup>1</sup> and Jayant K. Singh<sup>1,2\*</sup>

<sup>1</sup>Department of Chemical Engineering, Indian Institute of Technology Kanpur, Kanpur, 208016, India.

<sup>2</sup>Prescience Insilico Private Limited, Bangalore, 560049, India.

\*E-mail: [jayantks@iitk.ac.in](mailto:jayantks@iitk.ac.in)

<sup>†</sup>Equal contribution

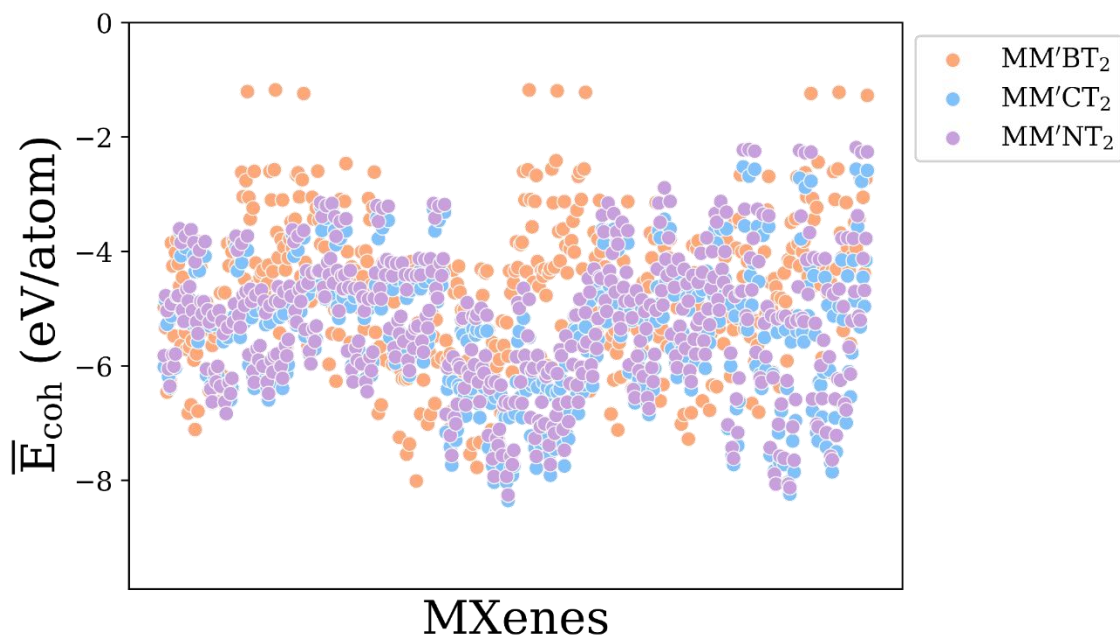

(a)

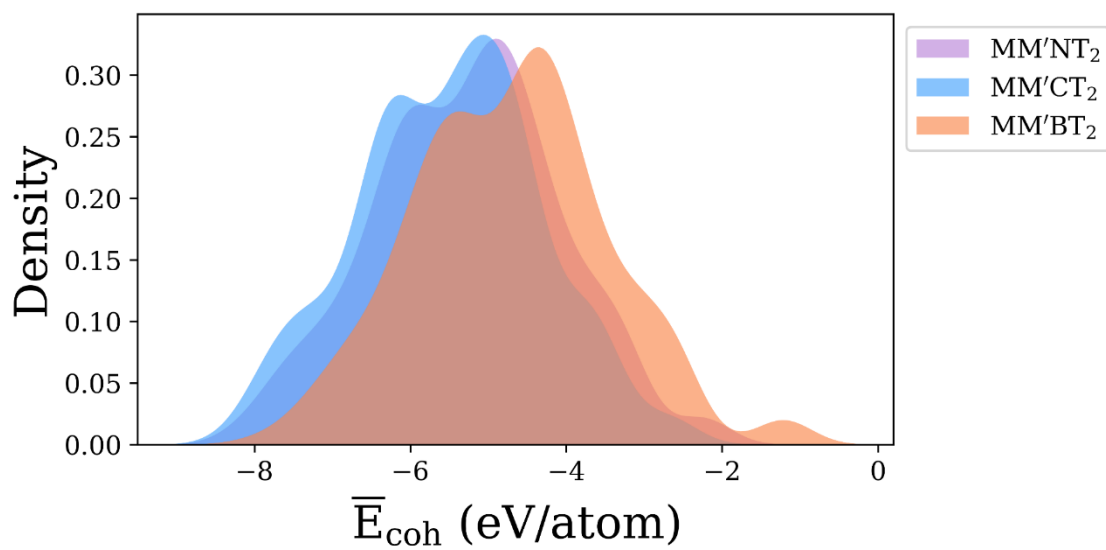

(b)

**Figure S1:** (a) Computed normalized cohesive energies  $\bar{E}_{\text{coh}}$  (eV/atom) and (b) corresponding distribution for the randomly selected 1125 MM'X<sub>2</sub>-type MXenes with respect to different X-layers (X = B, C or N).

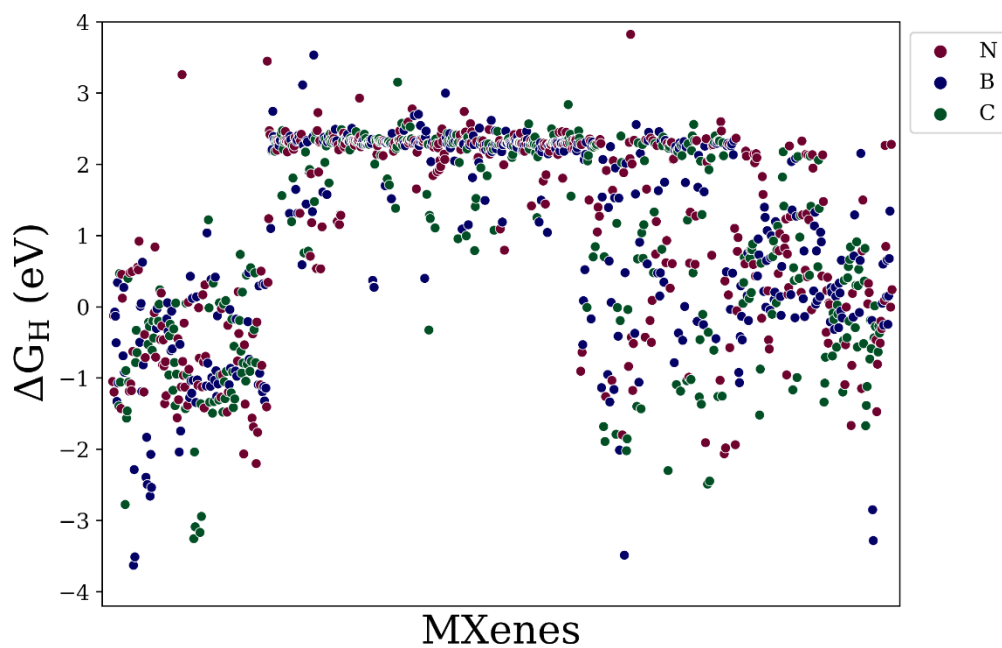

(a)

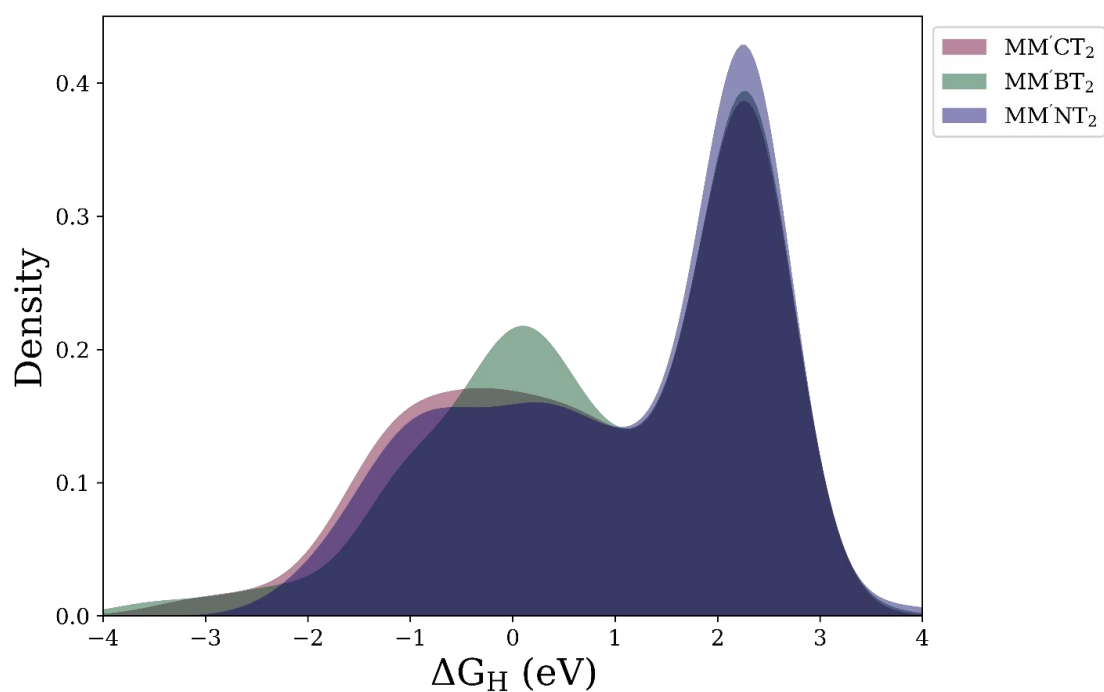

(b)

**Figure S2:** (a) DFT computed hydrogen adsorbed Gibbs free energies ( $\Delta G_H$ ) for randomly selected 1,125 MM'XT<sub>2</sub>-type MXenes and (b) their distribution with respect to different X-layers (X = B, C or N)

**Table S1:** List of primary features, including atomistic, structural and electronic indicators.

| SYMBOL                      | ATOMISTIC FEATURES         |
|-----------------------------|----------------------------|
| $W_X, W_M, W_{M'}, W_T$     | Atomic Weight              |
| $N_X, N_M, N_{M'}, N_T$     | Atomic Number              |
| $P_X, P_M, P_{M'}, P_T$     | Period number              |
| $G_X, G_M, G_{M'}, G_T$     | Group number               |
| $V_X, V_M, V_{M'}, V_T$     | Valence electron           |
| $IE_X, IE_M, IE_{M'}, IE_T$ | First Ionization Potential |
| $r_M, r_{M'}, r_T$          | Radius                     |
| $EA_M, EA_{M'}, EA_T$       | Electron Affinity          |
| $MP_M, MP_{M'}, MP_T$       | Melting Point              |
| $BP_M, BP_{M'}, BP_T$       | Boiling Point              |
| $\chi_M, \chi_{M'}$         | Electronegativity          |
| $X$                         | X-atom type                |
| $T$                         | Termination type           |

| SYMBOL                  | STRUCTURAL FEATURES                   |
|-------------------------|---------------------------------------|
| $W_{sur}, W$            | Surface Weight, Normalized            |
| $A_{sur}$               | Surface Area                          |
| $\rho_{sur}$            | Surface Density                       |
| $IE_D = IE_M - IE_{M'}$ | First Ionization Potential Difference |

| SYMBOL                                             | ELECTRONIC FEATURES         |
|----------------------------------------------------|-----------------------------|
| $LT$                                               | Layer Thickness             |
| $E_{coh}, \bar{E}_{coh}$                           | Cohesive Energy, Normalized |
| $l_{M-T}, l_{M'-T}, l_{M-X}, l_{M-X}$              | Bond lengths                |
| $d_{M-M}, d_{M-M'}, d_{T-T}, d_{T_1-T_2}, d_{X-X}$ | Distances (nearest)         |

|          |                                |
|----------|--------------------------------|
| $d_{NN}$ | Distance b/w Nearest Neighbors |
| $dbc$    | d-band center                  |
| $WF$     | Work function                  |

**Table S2:** Statistical functions for each of the  $\gamma$  properties that are used to expand the primary features

| Feature             | Description                                | Formula                                                     |
|---------------------|--------------------------------------------|-------------------------------------------------------------|
| $\bar{\gamma}$      | Average value                              | $\sum_{i=0}^n \gamma_i / N$                                 |
| $\tilde{\gamma}$    | Average weighted value                     | $\sum_{i=0}^n \gamma_i n_i / N$                             |
| $\gamma_{max}$      | Maximum value                              | $Max(\gamma_i)$                                             |
| $\gamma_{min}$      | Minimum value                              | $Min(\gamma_i)$                                             |
| $\gamma_{\sigma}$   | Standard deviation with respect to average | $\sqrt{\sum_{i=0}^n \frac{(\bar{\gamma} - \gamma_i)^2}{N}}$ |
| $\gamma_{\sigma^2}$ | Variance with respect to average           | $\sum_{i=0}^n \frac{(\bar{\gamma} - \gamma_i)^2}{N}$        |
| $\gamma^2$          | Squared value                              | $\gamma_i^2$                                                |

**Table S3:** Machine learning models and their description.

| <b>ABBREVIATION</b> | <b>MODEL</b>                | <b>TYPE</b>         | <b>DESCRIPTION</b>                                             |
|---------------------|-----------------------------|---------------------|----------------------------------------------------------------|
| <b>ABR</b>          | AdaBoost Regressor          | Ensemble            | ‘Adaptive Boosting’, fits a sequence of weak learning models   |
| <b>GBR</b>          | Gradient Boosting Regressor | Ensemble            | Builds additive model in forward stage-fashion                 |
| <b>KNR</b>          | K Neighbors Regressor       | Neighbors           | Based on K-nearest neighbors                                   |
| <b>KRR</b>          | Kernel Ridge                | Kernel Ridge        | Combines ridge (L2) penalty with kernel trick                  |
| <b>LAS</b>          | Lasso                       | Linear              | Trained with L1 penalty                                        |
| <b>RDG</b>          | Ridge Regression            | Linear Model        | Trained with L2 penalty                                        |
| <b>RFR</b>          | Random Forest Regressor     | Ensemble            | Meta estimator fitting a number of classifying decision trees  |
| <b>PLS</b>          | Partial Least Squares       | Cross Decomposition | Regularized linear regression, similar to Lasso                |
| <b>ENR</b>          | Elastic Net Regressor       | Linear              | Uses penalties from both lasso (L1) and ridge (L2) regressions |

**Table S4:** Mean absolute error (MAE) and coefficient of determination ( $R^2$ ) after cross validation for various feature subsets of nine different models.

| Model      | Feature Subset | MAE               | $R^2$              |
|------------|----------------|-------------------|--------------------|
| <b>ABR</b> | 1              | $0.635 \pm 0.055$ | $0.672 \pm 0.092$  |
|            | 2              | $0.724 \pm 0.074$ | $0.558 \pm 0.096$  |
|            | 3              | $0.709 \pm 0.079$ | $0.657 \pm 0.117$  |
|            | 1 + 2          | $0.698 \pm 0.063$ | $0.561 \pm 0.066$  |
|            | 1 + 3          | $0.597 \pm 0.055$ | $0.711 \pm 0.101$  |
|            | 2 + 3          | $0.602 \pm 0.092$ | $0.727 \pm 0.057$  |
|            | 1 + 2 + 3      | $0.767 \pm 0.027$ | $0.576 \pm 0.034$  |
| <b>GBR</b> | 1              | $0.512 \pm 0.105$ | $0.726 \pm 0.154$  |
|            | 2              | $0.662 \pm 0.071$ | $0.546 \pm 0.069$  |
|            | 3              | $0.585 \pm 0.123$ | $0.701 \pm 0.068$  |
|            | 1 + 2          | $0.675 \pm 0.06$  | $0.549 \pm 0.086$  |
|            | 1 + 3          | $0.472 \pm 0.052$ | $0.772 \pm 0.098$  |
|            | 2 + 3          | $0.514 \pm 0.077$ | $0.776 \pm 0.083$  |
|            | 1 + 2 + 3      | $0.424 \pm 0.05$  | $0.771 \pm 0.066$  |
| <b>KRR</b> | 1              | $0.592 \pm 0.076$ | $0.712 \pm 0.13$   |
|            | 2              | $0.715 \pm 0.043$ | $0.546 \pm 0.068$  |
|            | 3              | $0.799 \pm 0.144$ | $-1.205 \pm 4.603$ |
|            | 1 + 2          | $0.666 \pm 0.049$ | $0.589 \pm 0.045$  |
|            | 1 + 3          | $0.995 \pm 0.39$  | $-0.502 \pm 2.228$ |

|            |           |                   |                    |
|------------|-----------|-------------------|--------------------|
|            | 2 + 3     | $0.77 \pm 0.107$  | $0.573 \pm 0.096$  |
|            | 1 + 2 + 3 | $0.696 \pm 0.085$ | $0.18 \pm 0.077$   |
| <b>KNR</b> | 1         | $1.25 \pm 0.126$  | $0.003 \pm 0.161$  |
|            | 2         | $0.812 \pm 0.039$ | $0.401 \pm 0.091$  |
|            | 3         | $1.449 \pm 0.101$ | $-0.247 \pm 0.119$ |
|            | 1 + 2     | $0.921 \pm 0.039$ | $0.239 \pm 0.08$   |
|            | 1 + 3     | $1.453 \pm 0.161$ | $-0.286 \pm 0.212$ |
|            | 2 + 3     | $1.458 \pm 0.135$ | $-0.268 \pm 0.135$ |
|            | 1 + 2 + 3 | $1.319 \pm 0.066$ | $0.191 \pm 0.09$   |
| <b>LAS</b> | 1         | $0.512 \pm 0.105$ | $0.726 \pm 0.154$  |
|            | 2         | $1.017 \pm 0.067$ | $0.294 \pm 0.066$  |
|            | 3         | $1.096 \pm 0.081$ | $0.247 \pm 0.129$  |
|            | 1 + 2     | $0.728 \pm 0.088$ | $-0.541 \pm 0.083$ |
|            | 1 + 3     | $0.787 \pm 0.071$ | $0.546 \pm 0.106$  |
|            | 2 + 3     | $1.062 \pm 0.129$ | $0.291 \pm 0.074$  |
|            | 1 + 2 + 3 | $0.639 \pm 0.047$ | $0.614 \pm 0.068$  |
| <b>RFR</b> | 1         | $0.507 \pm 0.074$ | $0.728 \pm 0.094$  |
|            | 2         | $0.709 \pm 0.068$ | $0.472 \pm 0.102$  |
|            | 3         | $0.571 \pm 0.067$ | $0.724 \pm 0.086$  |
|            | 1 + 2     | $0.714 \pm 0.061$ | $0.459 \pm 0.094$  |
|            | 1 + 3     | $0.447 \pm 0.085$ | $0.776 \pm 0.09$   |

|            |           |                   |                   |
|------------|-----------|-------------------|-------------------|
|            | 2 + 3     | $0.493 \pm 0.108$ | $0.781 \pm 0.061$ |
|            | 1 + 2 + 3 | $0.382 \pm 0.025$ | $0.806 \pm 0.061$ |
| <b>RDG</b> | 1         | $0.586 \pm 0.092$ | $0.711 \pm 0.087$ |
|            | 2         | $0.713 \pm 0.063$ | $0.547 \pm 0.06$  |
|            | 3         | $0.609 \pm 0.053$ | $0.674 \pm 0.155$ |
|            | 1 + 2     | $0.668 \pm 0.061$ | $0.587 \pm 0.052$ |
|            | 1 + 3     | $0.622 \pm 0.117$ | $0.554 \pm 0.46$  |
|            | 2 + 3     | $0.605 \pm 0.099$ | $0.679 \pm 0.075$ |
|            | 1 + 2 + 3 | $0.563 \pm 0.039$ | $0.686 \pm 0.058$ |
| <b>ENR</b> | 1         | $0.693 \pm 0.068$ | $0.633 \pm 0.05$  |
|            | 2         | $0.993 \pm 0.066$ | $0.32 \pm 0.047$  |
|            | 3         | $1.084 \pm 0.089$ | $0.279 \pm 0.087$ |
|            | 1 + 2     | $0.717 \pm 0.034$ | $0.544 \pm 0.043$ |
|            | 1 + 3     | $0.701 \pm 0.084$ | $0.622 \pm 0.095$ |
|            | 2 + 3     | $1.034 \pm 0.087$ | $0.328 \pm 0.109$ |
|            | 1 + 2 + 3 | $0.634 \pm 0.042$ | $0.618 \pm 0.069$ |
| <b>PLS</b> | 1         | $0.582 \pm 0.078$ | $0.714 \pm 0.077$ |
|            | 2         | $0.914 \pm 0.062$ | $0.371 \pm 0.083$ |
|            | 3         | $1.025 \pm 0.071$ | $0.342 \pm 0.087$ |
|            | 1 + 2     | $0.682 \pm 0.071$ | $0.575 \pm 0.054$ |
|            | 1 + 3     | $0.637 \pm 0.063$ | $0.667 \pm 0.127$ |

|  |           |                   |                   |
|--|-----------|-------------------|-------------------|
|  | 2 + 3     | $0.925 \pm 0.064$ | $0.43 \pm 0.113$  |
|  | 1 + 2 + 3 | $0.704 \pm 0.062$ | $0.569 \pm 0.068$ |

Where,

Set 1 = Atomistic Features

Set 2 = Surface Features (Structural + Electronic)

Set 3 = Statistical Features

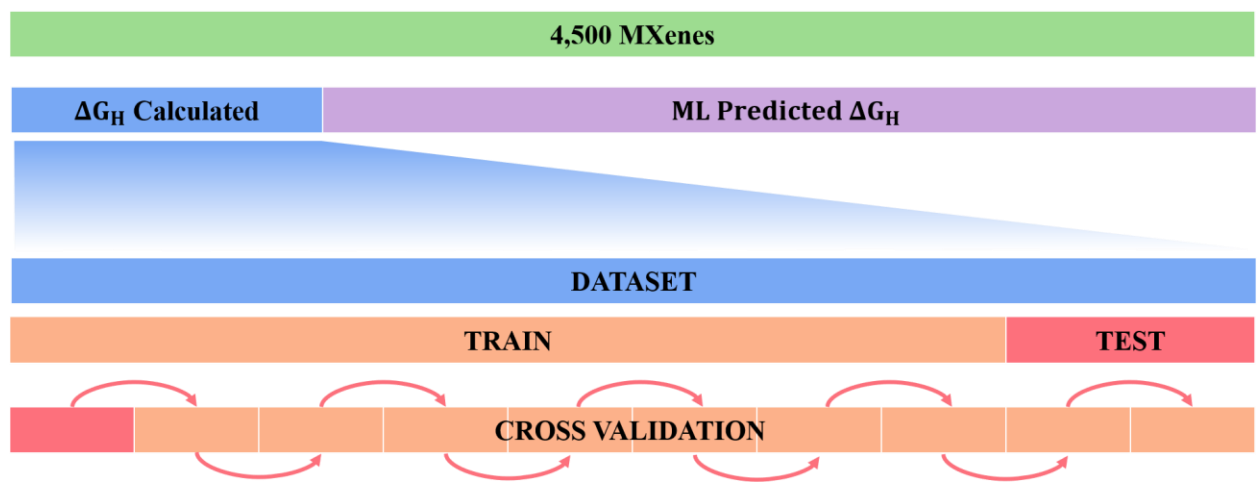

**Figure S3:** Pictorial representation of data distribution for Training-Testing and 10-fold Cross Validation.

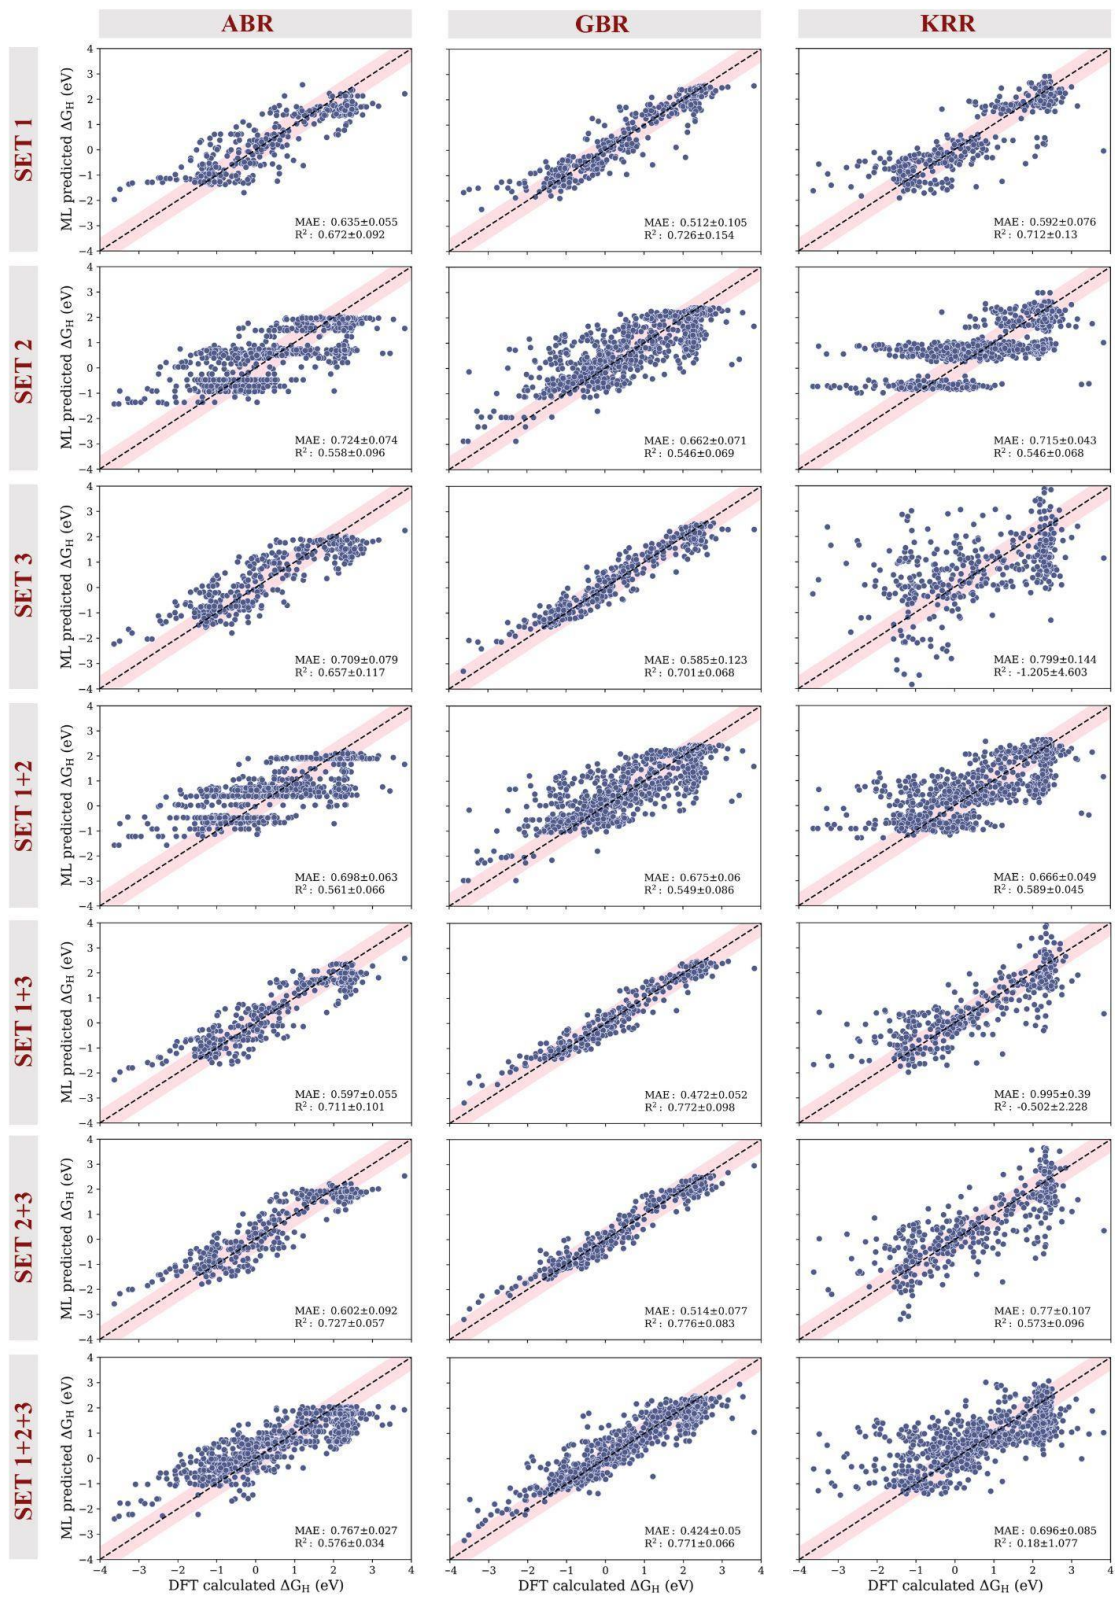

(a)

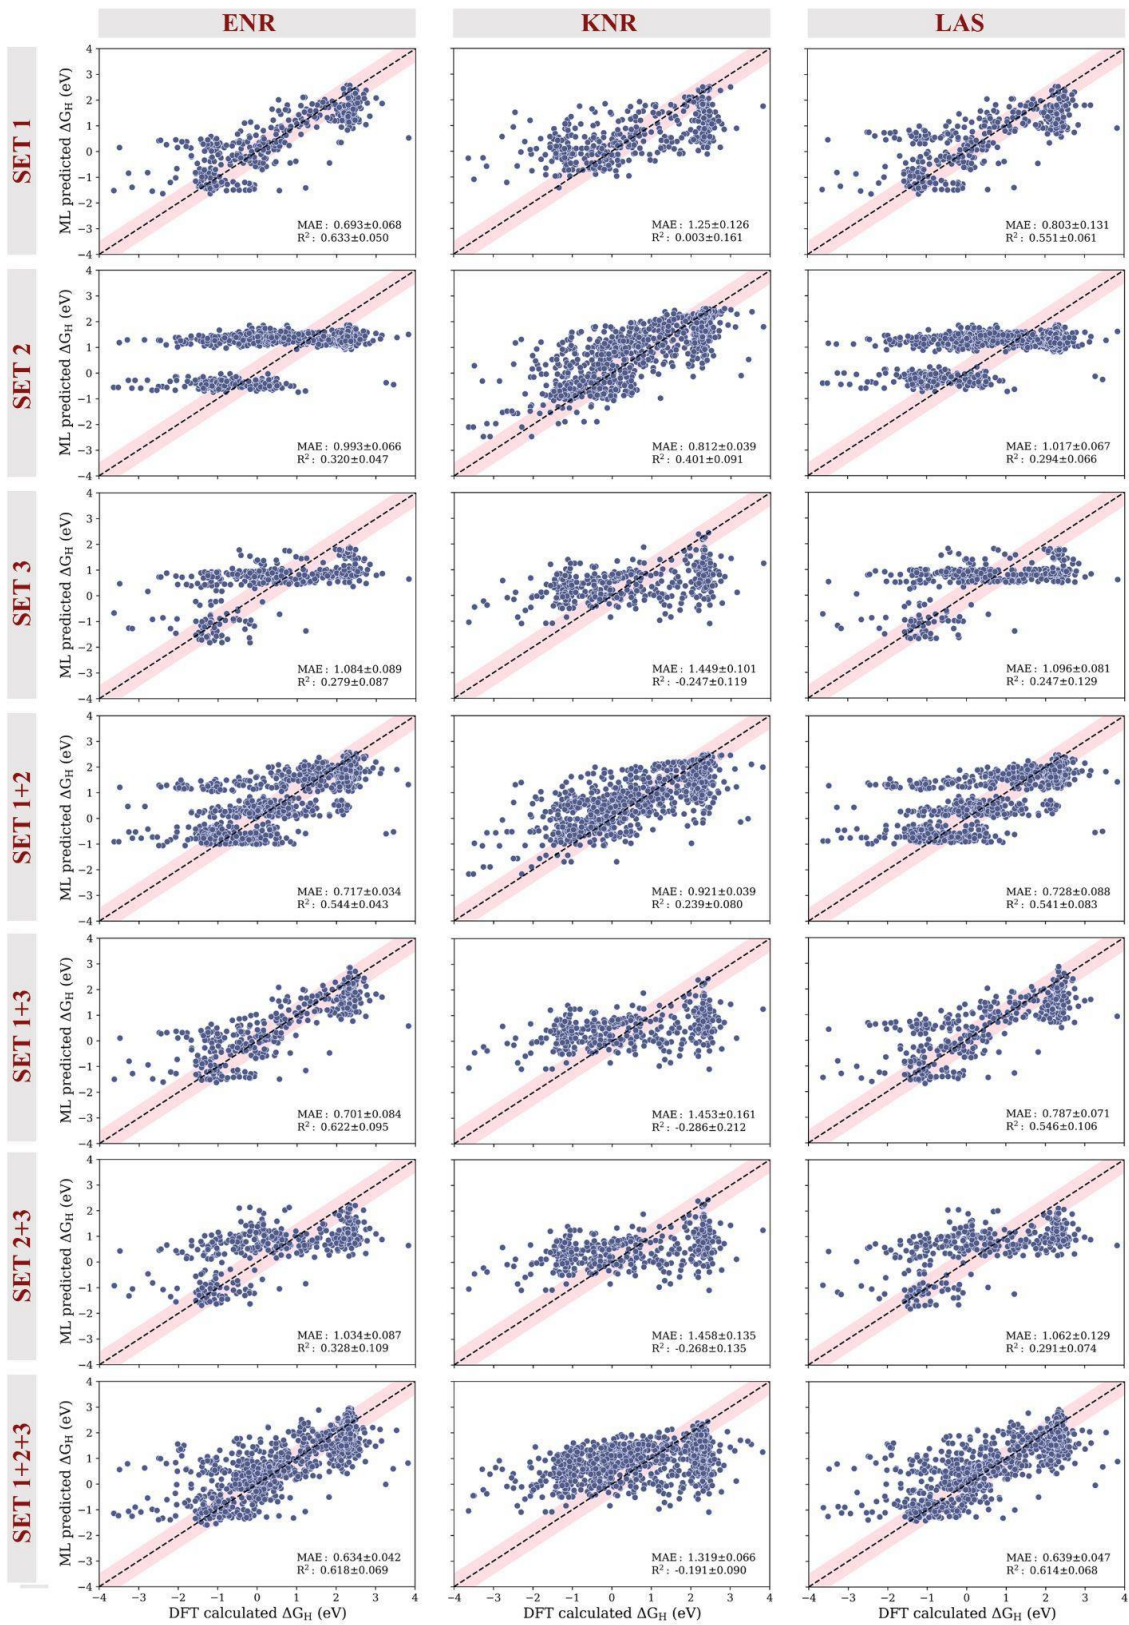

(b)

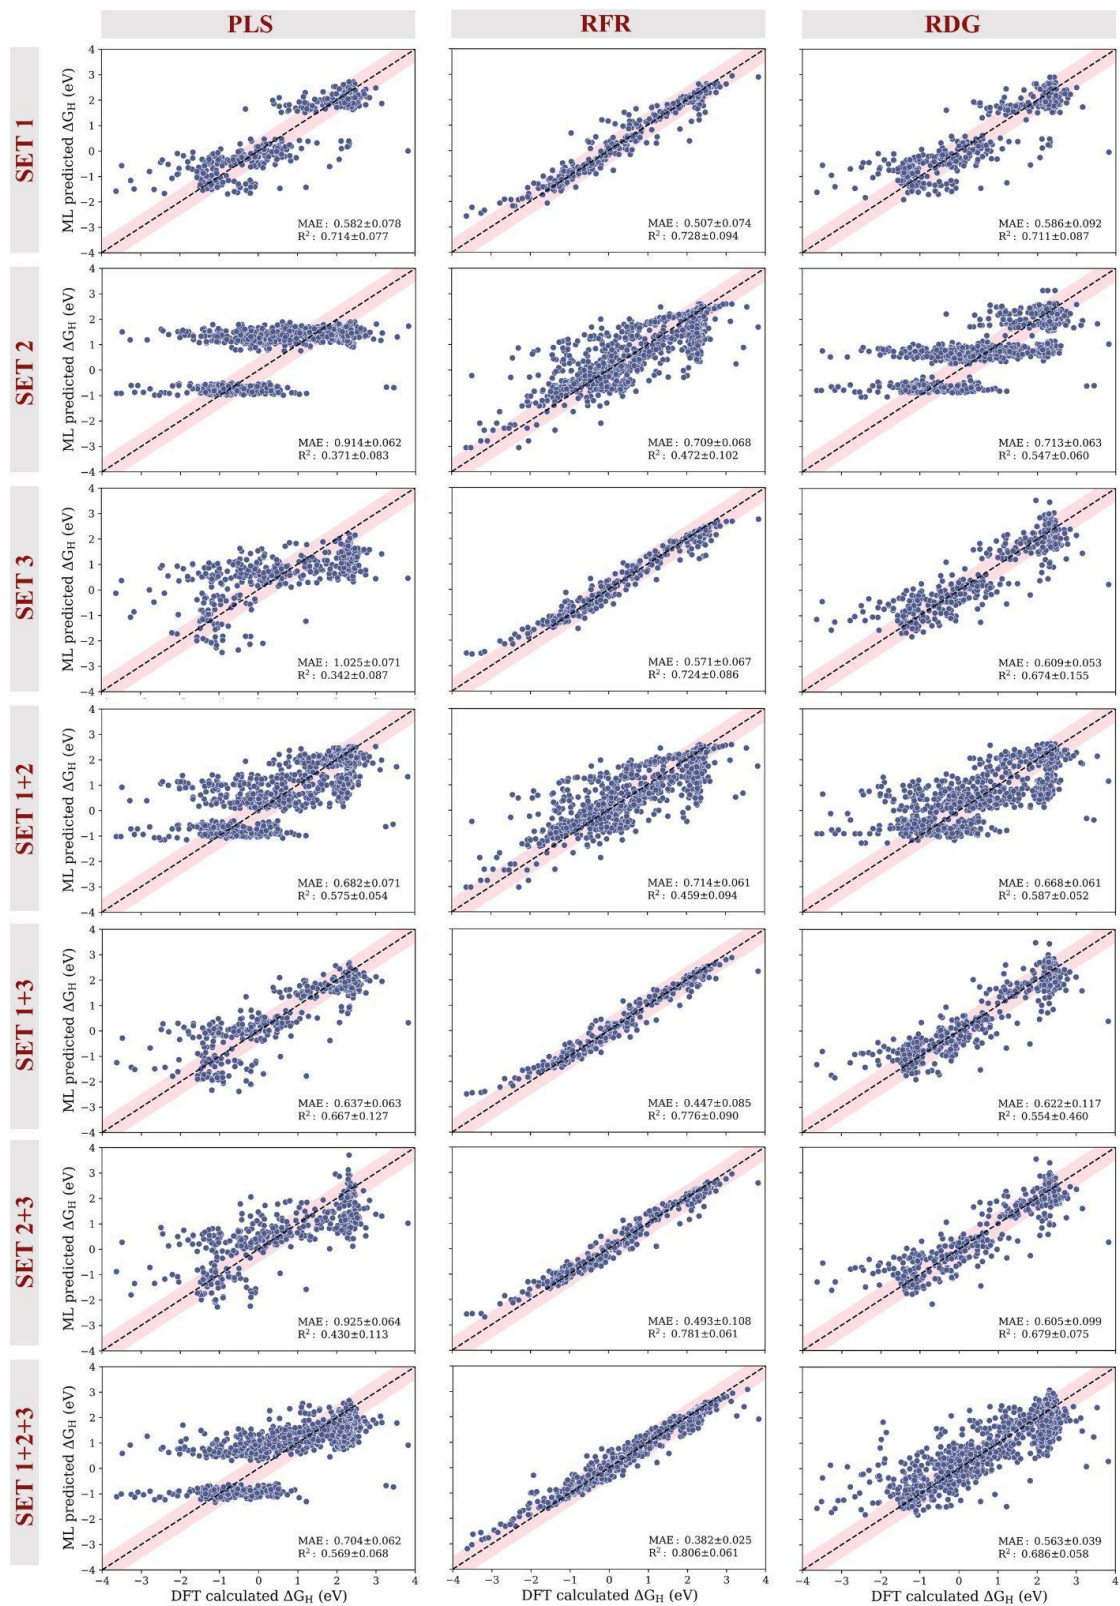

(c)

**Figure S4:** Parity plots for various sets using different ML models.

**Table S5:** Mean absolute error (MAE) and coefficient of determination ( $R^2$ ) for the training and testing data of set 1 + 2 + 3 using different ML models.

| <b>Models</b> | <b>Train MAE</b> | <b>Test MAE</b> | <b>Train <math>R^2</math></b> | <b>Test <math>R^2</math></b> |
|---------------|------------------|-----------------|-------------------------------|------------------------------|
| <b>ABR</b>    | 0.666            | 0.702           | 0.701                         | 0.574                        |
| <b>GBR</b>    | 0.294            | 0.421           | 0.913                         | 0.753                        |
| <b>KNR</b>    | 1.083            | 1.342           | 0.215                         | 0.005                        |
| <b>KRR</b>    | 0.707            | 0.625           | 0.561                         | 0.621                        |
| <b>LAS</b>    | 0.647            | 0.578           | 0.619                         | 0.668                        |
| <b>RDG</b>    | 0.52             | 0.568           | 0.746                         | 0.672                        |
| <b>RFR</b>    | 0.144            | 0.388           | 0.973                         | 0.776                        |
| <b>PLS</b>    | 0.717            | 0.647           | 0.576                         | 0.592                        |
| <b>ENR</b>    | 0.642            | 0.573           | 0.629                         | 0.676                        |

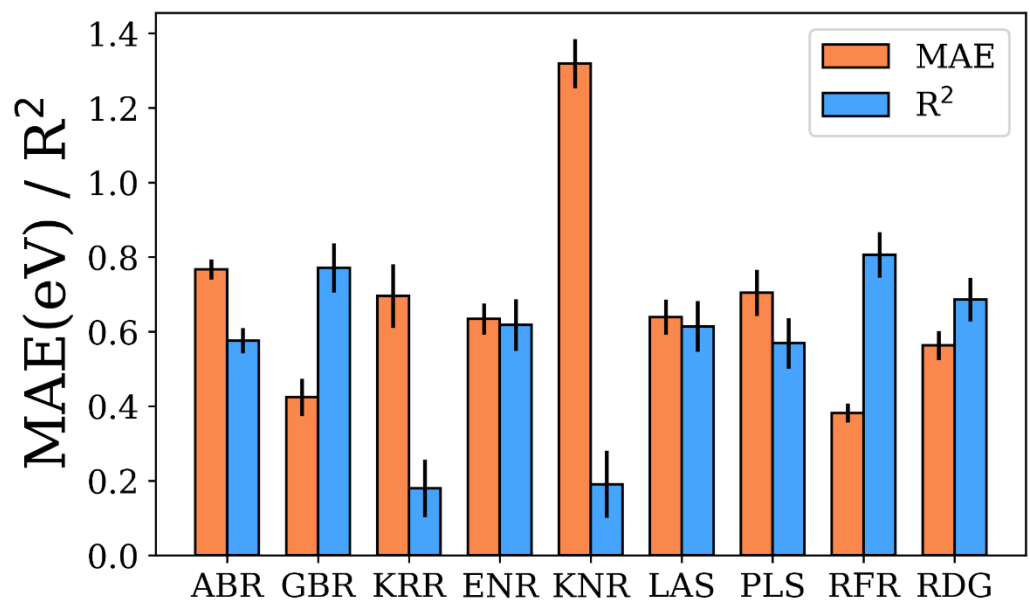

**Figure S5:** Mean absolute error (MAE) and coefficient of determination ( $R^2$ ) after cross validation for set 1 + 2 + 3 using different ML models.

**Table S6:** List of hyperparameters selected after using Randomized Search CV.

| Method                   | Hyperparameters                                                                                           |
|--------------------------|-----------------------------------------------------------------------------------------------------------|
| <b>Random Forest</b>     | n_estimators = 1000, min_samples_leaf = 2, max_features = 15, max_depth = 500, bootstrap = True           |
| <b>Gradient Boosting</b> | n_estimators = 400, min_samples_leaf = 10, max_features = 'sqrt', max_depth = 1000, learning_rate = 0.015 |

**Table S7:** Mean absolute error (MAE) and coefficient of determination ( $R^2$ ) for RFR and GBR models after RFE-HO parameterization.

| Model      | Scoring parameter | Feature Set Selection | Recursive Feature Elimination | Hyperparameter Optimization |
|------------|-------------------|-----------------------|-------------------------------|-----------------------------|
| <b>RFR</b> | MAE               | 0.382                 | 0.376                         | 0.374                       |
|            | $R^2$             | 0.806                 | 0.811                         | 0.817                       |
| <b>GBR</b> | MAE               | 0.424                 | 0.384                         | 0.371                       |
|            | $R^2$             | 0.771                 | 0.810                         | 0.814                       |

**Table S8:** Top seven features for RFR model after RFE-HO parameterization

| Symbols          | Features                           |
|------------------|------------------------------------|
| $EA_T$           | Electron Affinity of termination   |
| $V_T$            | Valence electron of termination    |
| $WF$             | Work Function                      |
| $MP_T$           | Melting Point of Termination       |
| $LT$             | Layer Thickness                    |
| $l_{M-X}$        | Bond length b/w Metal 1 and X-atom |
| $\overline{dbc}$ | d-band center average value        |

**Table S9:** Top seven features for GBR model after RFE-HO parameterization

| Symbols      | Features                                       |
|--------------|------------------------------------------------|
| $EA_T$       | Electron Affinity of termination               |
| $V_T$        | Valence electron of termination                |
| $WF$         | Work Function                                  |
| $l_{M-T}$    | Bond length b/w Metal1 and Termination         |
| $d_{X-X}$    | X-atoms' (nearest) distance                    |
| $\chi_T$     | Electronegativity of termination               |
| $d_{M-M'}^2$ | Metal1-Metal2 (nearest) distance squared value |

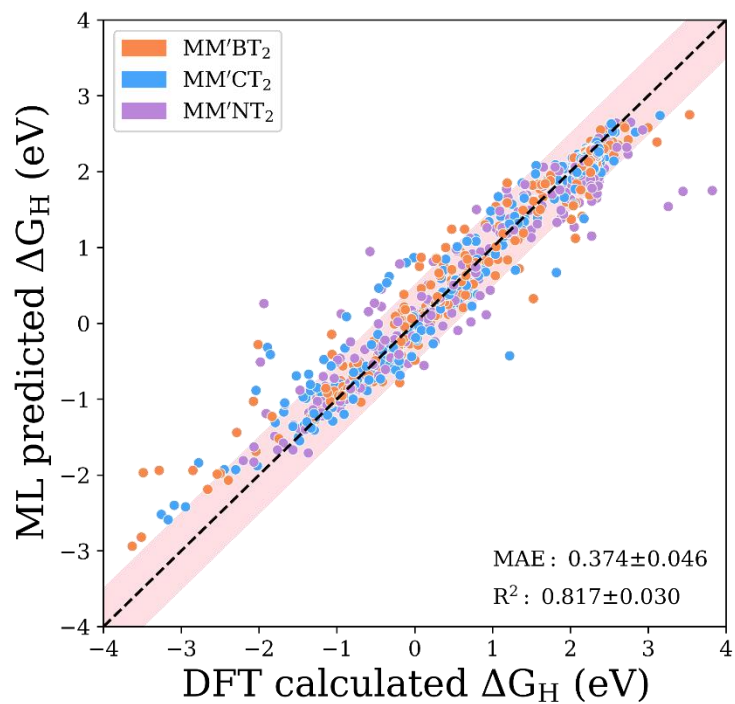

(a)

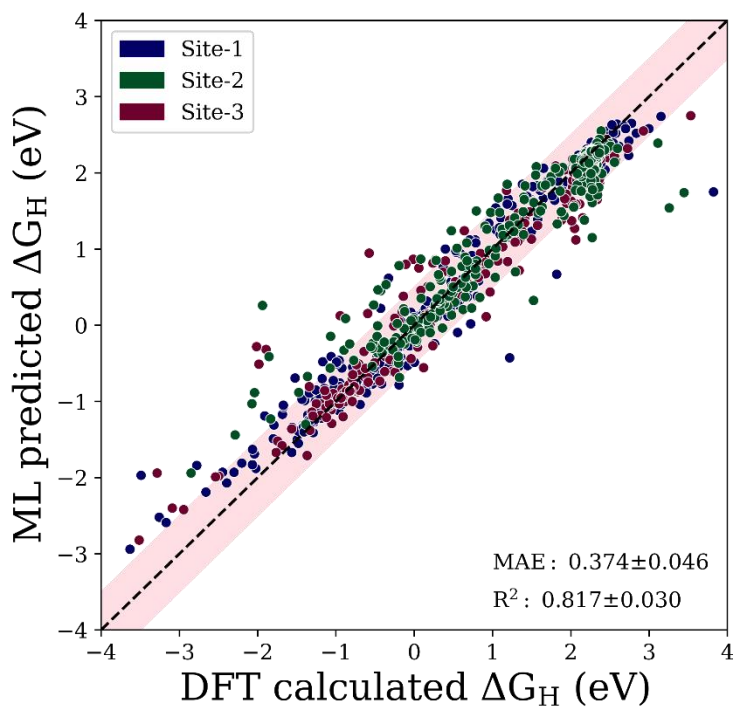

(b)

**Figure S6:** Parity plots of RFR model after RFE-HO parameterization with respect to (a) X-layers (X = B, C or N) and (b) adsorption sites.

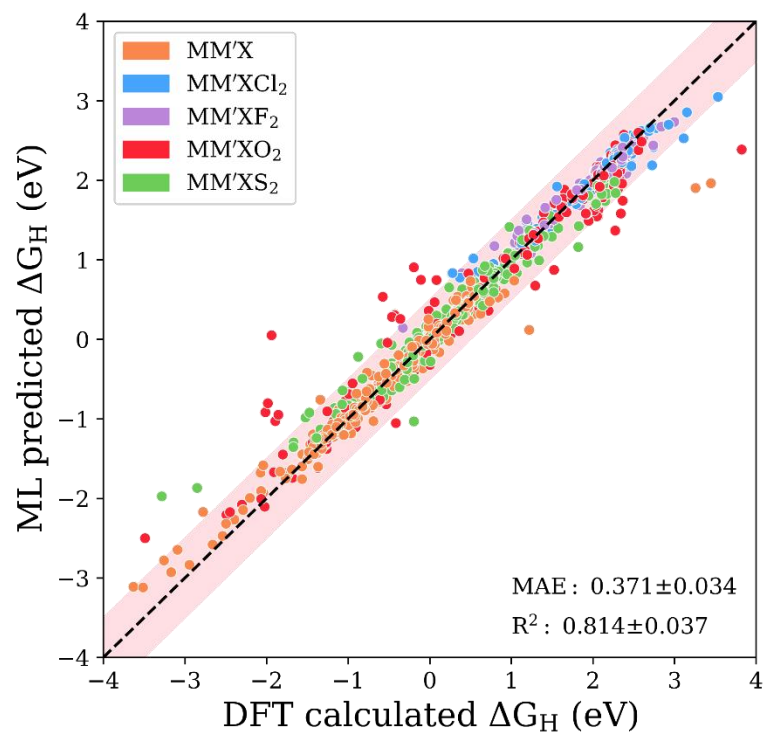

**Figure S7:** Predicted vs actual  $\Delta G_H$  GBR using RFE-HO parameterization in the best testing prediction process. The pink-shaded region indicates a deviation of up to 0.5 eV.

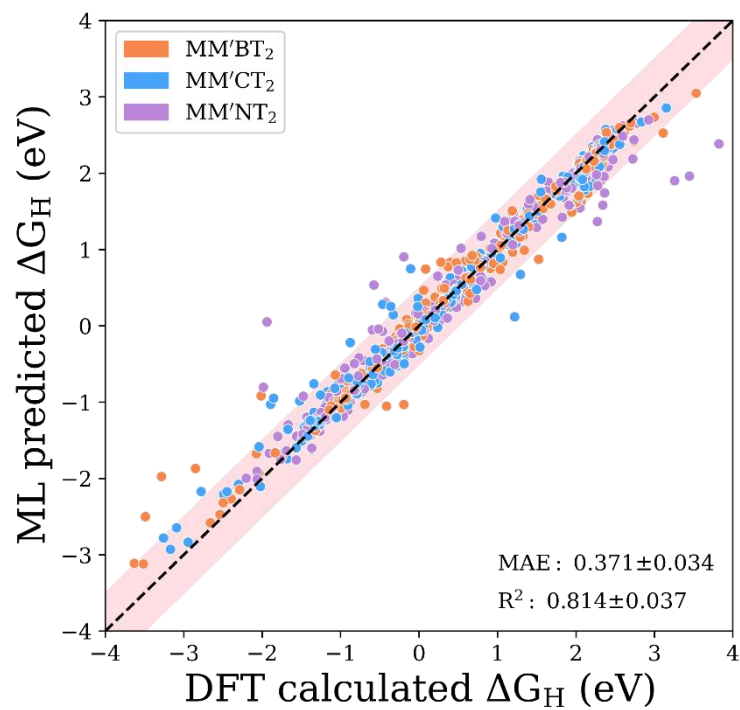

(a)

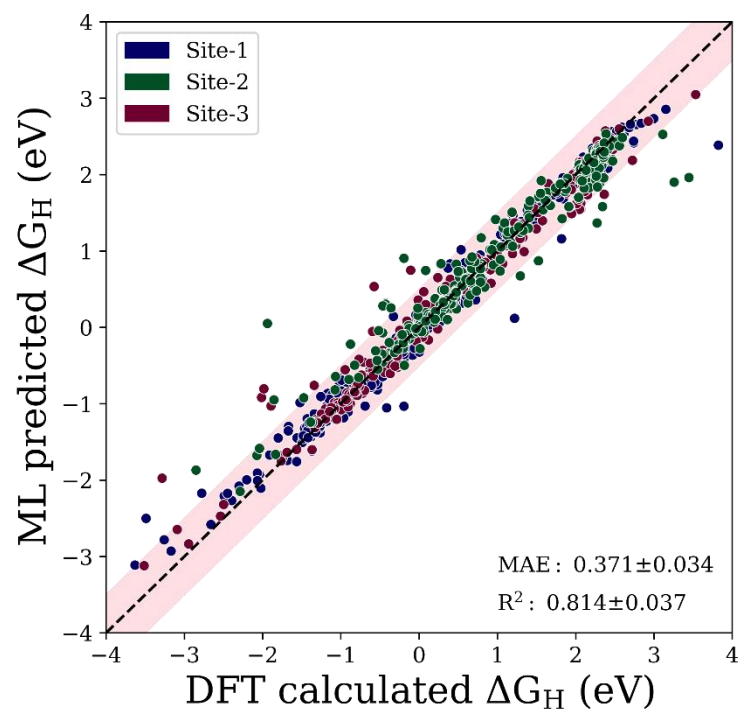

(b)

**Figure S8:** Parity plots of GBR model after RFE-HO parameterization with respect to (a) X-layers (X = B, C or N) and (b) adsorption sites.

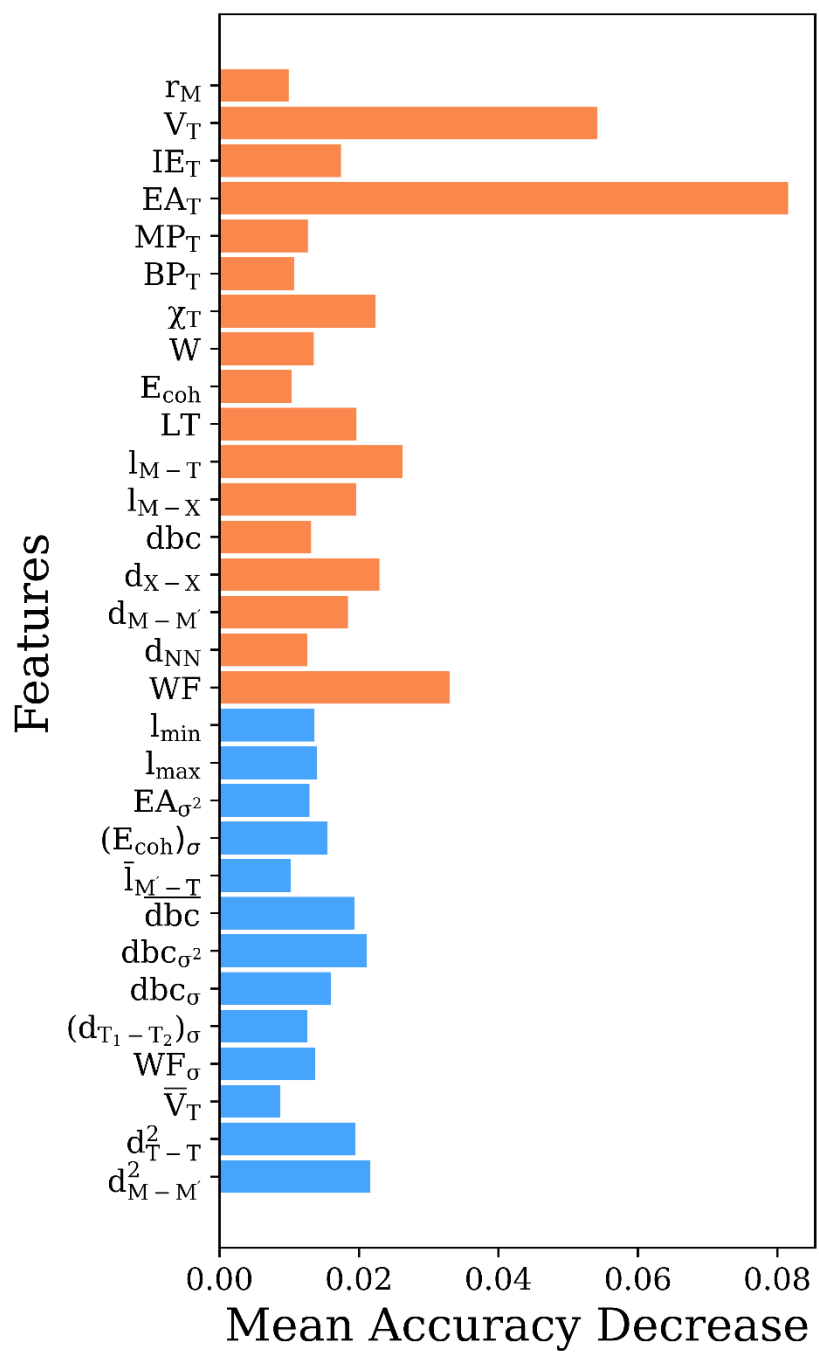

**Figure S9:** Important features GBR model using RFE-HO parameterization that were evaluated via 10-fold cross-validation. Orange and blue colors indicate primary and statistical features respectively.

**Table S10:** Top MM'XT<sub>2</sub>-type MXenes with better stability and high HER activity predicted using RFR Model after RFE-HO parameterization.

| <b>MXenes</b>          | $\bar{E}_{\text{coh}}$ | ML Predicted $\Delta G_{\text{H}}$ |
|------------------------|------------------------|------------------------------------|
| MoTiCO <sub>2</sub> -1 | -7.265                 | 0.051                              |
| MoVBO <sub>2</sub> -1  | -7.013                 | 0.094                              |
| NbCrBO <sub>2</sub> -1 | -7.108                 | -0.078                             |
| NbMoCO <sub>2</sub> -1 | -7.930                 | -0.050                             |
| TiNbCO <sub>2</sub> -1 | -7.579                 | 0.026                              |
| VNbNO <sub>2</sub> -1  | -7.909                 | -0.087                             |
| VTiBO <sub>2</sub> -1  | -6.609                 | -0.018                             |
| YNbNO <sub>2</sub> -1  | -7.747                 | -0.002                             |
| CrCrN-2                | -7.090                 | 0.082                              |
| MoCrN-2                | -7.559                 | -0.062                             |
| NbCrB-2                | -6.790                 | 0.072                              |
| NbCrC-2                | -7.613                 | 0.002                              |
| NbMoC-2                | -8.065                 | -0.059                             |
| NbTiC-2                | -7.062                 | 0.022                              |
| NbTiN-2                | -7.308                 | -0.094                             |
| NbVN-2                 | -7.849                 | -0.047                             |
| TiMoC-2                | -7.018                 | -0.040                             |
| TiNbC-2                | -7.062                 | 0.019                              |
| TiVC-2                 | -6.570                 | -0.096                             |
| VMoB-2                 | -6.848                 | -0.040                             |
| VNbB-2                 | -6.818                 | 0.063                              |
| VNbC-2                 | -7.640                 | 0.006                              |
| VVC-2                  | -7.215                 | -0.090                             |
| VVN-2                  | -7.500                 | -0.039                             |
| VYN-2                  | -6.610                 | -0.042                             |
| YYNO <sub>2</sub> -2   | -6.819                 | -0.036                             |
| CrMoBO <sub>2</sub> -3 | -6.823                 | -0.012                             |
| CrVNO <sub>2</sub> -3  | -7.297                 | 0.004                              |

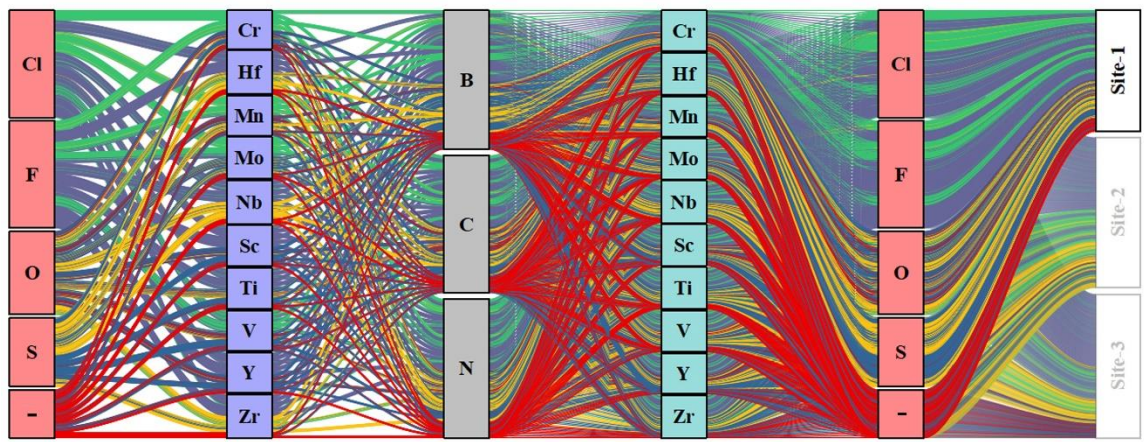

(a)

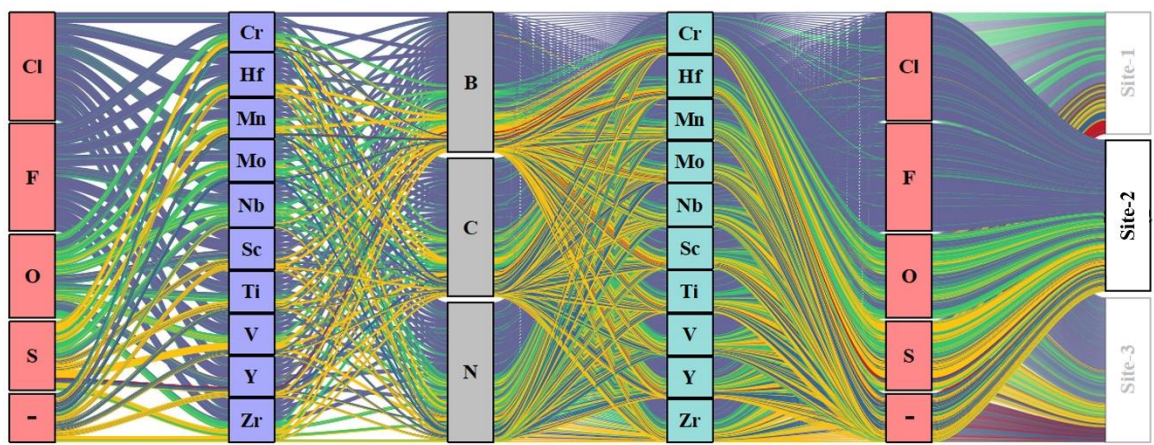

(b)

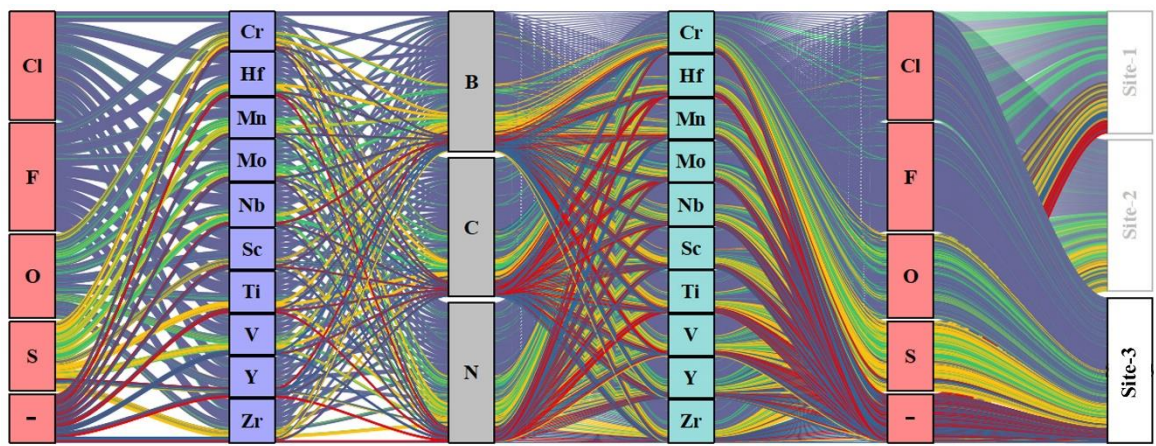

(c)

**Figure S10:** Alluvial Diagram showing (a) Site-1, (b) Site-2, and (c) Site-3 of ML Predicted  $\Delta G_H$  of 4,500 MXenes. Blue, red and yellow color links represent positive, negative and close to zero  $\Delta G_H$  value respectively.
